# Supplementary material for: SynthesizRR: Generating Diverse Datasets with Retrieval Augmentation
Source: arXiv:2405.10040 source file (2024-11-13)
Supplement: Supplementary file 1 [file baselines-description.tex]

Here, we explore how \ours{} directly compares to prior work on synthesis of popular datasets. We compare against six prior approaches: 

\insection[]{\ZeroGen{} \cite{Ye2022ZeroGenEZ}:} a simple approach which uses zero-shot generation from \GPTTwoXL{} under different prompting schemes. For certain tasks like \IMDb{} and \SST, the authors occasionally seed the prompt with a previously-generated movie name (described subsequently).

% \insection[]{\ProGen{} \cite{ye-etal-2022-progen}:} generates a small synthetic dataset, then uses a student model along with an influence function to highlight high-quality generations. These are used as in-context examples for another round of generation.

\insection[]{\SunGen{} \cite{gao2023selfguided}:} uses the \ZeroGen{} strategy to generate a large synthetic dataset (200k rows). Then, uses a custom bi-level optimization algorithm (involving the student model) to determine instance-weights of each synthetic example. 

\insection[]{\ReGen{} \cite{yu-etal-2023-regen}:} performs multi-round filtering of retrieved results using 2 BERT models; one trained for retrieval, and one classifier. Use consistency between these models to filter noisy data. 

\insection[]{\LetsSynth{} \cite{wang-etal-2023-lets}:} Constructs a ``seed dataset'' (different from ours) and trains a student model. Then, extrapolate errors using an LLM and synthesizes additional data. We combine this with the seed data and repeat the process.

\insection[]{\AttrPrompt{} \cite{yu2023large}:} a method focused on improving diversity and unbiasedness of generated datasets. Prompts a powerful LLM like \ChatGPT{} with different attributes, each along different dimensions. Attributes are extracted from a human-in-the-loop analysis of task using \ChatGPT{}.

We note that zero shot generation and few-shot generation has already been compared in \autoref{tab:student-deb}, so we do not include it here.

We benchmark four classification tasks which are popular in prior work: \YelpPolarity{} \citep{zhang2015character}, \IMDb{} \cite{maas-etal-2011-learning}, \SST{} \cite{socher-etal-2013-recursive} and \AGNews{} \citep{zhang2015character}. The first three tasks are binary sentiment analysis, whereas the last is multi-class topic classification.

For the content sourcing stage of \ours, we retrieve documents from the following corpora:
\begin{itemize}
\item \YelpPolarity: to generate positive and negative reviews about businesses, we retrieve from the \YelpDataset{} corpus \cite{yelpcorpus} which contains details of 150k businesses. Each document contains the the name, address, and various tags and boolean attributes for a single business.
\item \IMDb{} and \SST: to generate movie reviews, we retrieve from the \CMUMovies{} corpus \cite{bamman-etal-2013-learning}, which contains 42k plot summaries. Each document is a plot summary for a single movie.
\item \AGNews: we use \RealNewsDominant{} from \autoref{tab:corpus}.
\end{itemize}

We note that the \CMUMovies{} and \YelpDataset{} corpora are between one to three orders of magnitude smaller than corpora in \autoref{tab:corpus}, thus it helps us evaluate \ours{} with smaller corpora. We include two different retrieval approaches: \Contriever{} (semantic match) and \BM{} (lexical match).

Following \citet{yu2023large}, we generate 6,000 rows using the \ours{} \RetrICL{} variant described in Algorithm~\ref{alg:synthesizrr}. We generate an equal number of examples for each class. We calculate intrinsic metrics Self-BLEU-5, MAUVE and Entity Entropy as described in \S\ref{sec:expt-setup}. 

Prior work often generates much larger datasets (20k to 200k examples) and uses different student model hyperparameters. Intrinsic evaluations of dataset quality are also seldom reported. This makes it difficult to fairly compare results from previous papers. Thus, we reproduce results ourselves by using synthetic datasets released by the authors, after subsampling to 6,000 examples. We report distillation results in \autoref{tab:baselines-student} and intrinsic metrics in \autoref{tab:baselines-intrinsic}.
